# Supplementary material for: Why scholars are diagramming neural network models
Source: arXiv:2104.14811 source file (2022-06-10)
Supplement: Supplementary file 1 [file appendix.tex]

This appendix includes example diagrams from ACL 2018 for each mental model type as outlined in Figure \ref{fig:schematics}. Figures \ref{fig:function2} and \ref{fig:purpose1} are from the same paper, suggesting the author had different representational priorities for different aspects of the system. 

\begin{figure}[htp]
    \centering
    \includegraphics[scale=0.5]{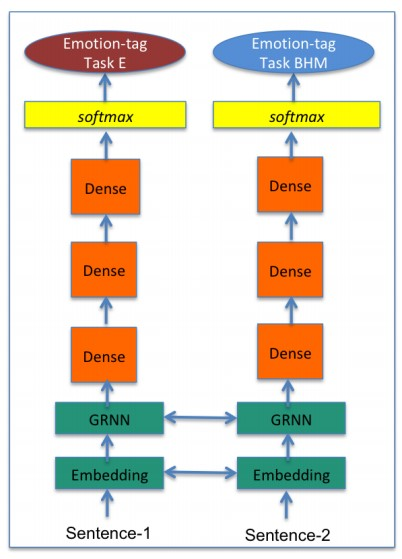}
    \caption{Form diagram, showing system components, used by \cite{tafreshi2018emotion}}
    \label{fig:form1}
\end{figure}

\begin{figure}[htp]
    \centering
    \includegraphics[scale=0.4]{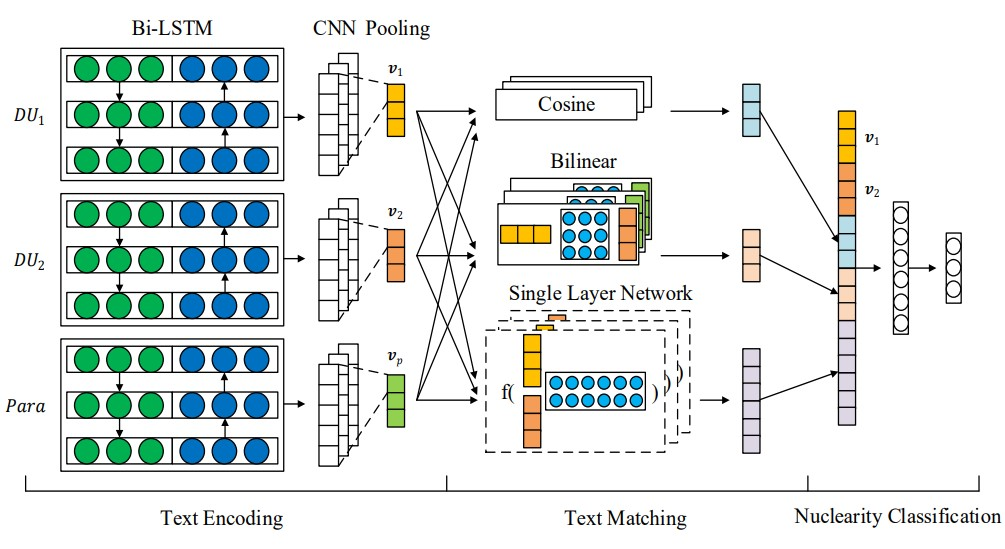}
    \caption{Function diagram, using verbs to label, used by \cite{xu2018employing}}
    \label{fig:function1}
\end{figure}

\begin{figure}[htp]
    \centering
    \includegraphics[scale=0.4]{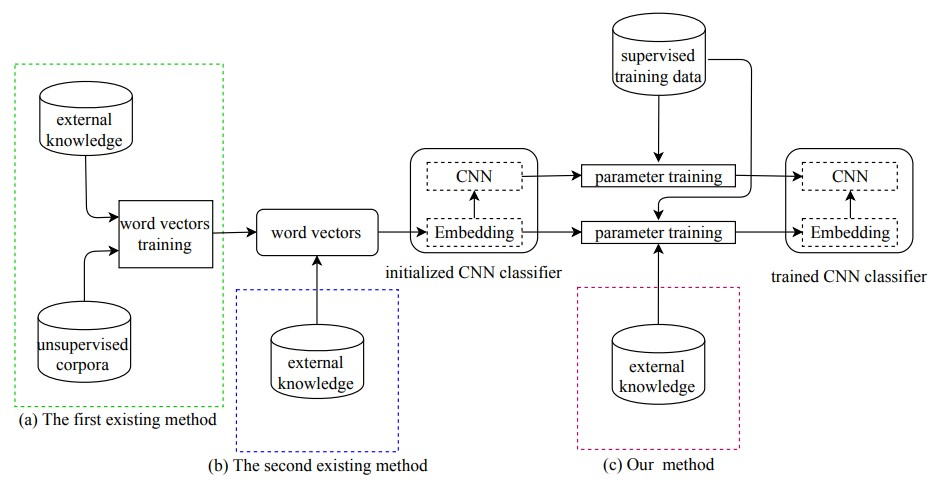}
    \caption{Function diagram, using verbs to label inside blocks, used by \cite{ye2018encoding}}
    \label{fig:function2}
\end{figure}
%In this one, it is not clear whether the absence of ellipsis means they are 4-vectors: A Position-aware Bidirectional Attention Network for Aspect-level Sentiment Analysis – Shuqin Gu, Lipeng Zhang, Yuexian Hou and Yin Song. 

\begin{figure}[htp]
    \centering
    \includegraphics[scale=0.5]{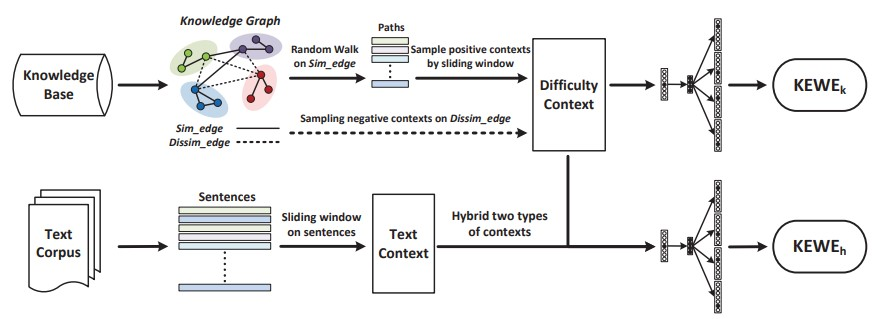}
    \caption{State, with process noun on an arrow, used by \cite{jiang2018enriching}}
    \label{fig:state1}
\end{figure}

\begin{figure}[htp]
    \centering
    \includegraphics[scale=0.45]{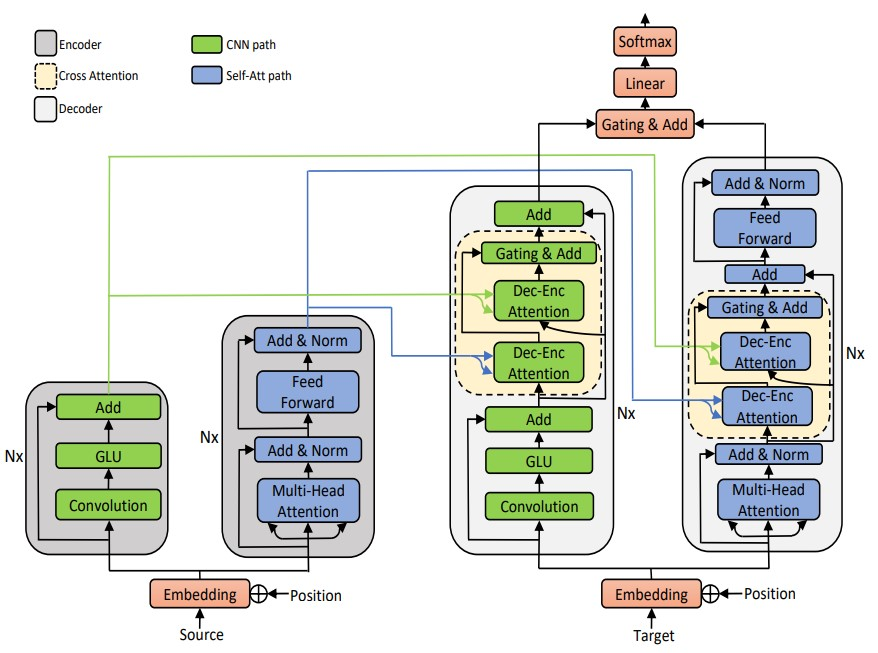}
    \caption{State, with process noun on in a box (e.g. "Add \& Norm"), used by \cite{song2018double}}
    \label{fig:state2}
\end{figure}

\begin{figure}[htp]
    \centering
    \includegraphics[scale=0.5]{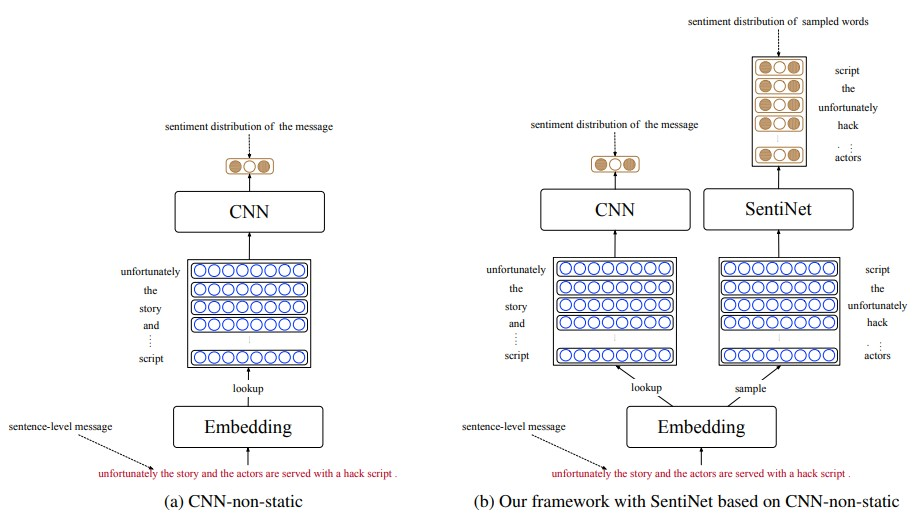}
    \caption{Purpose diagram, focusing on components and example data, used by \cite{ye2018encoding}}
    \label{fig:purpose1}
\end{figure}
